# Supplementary material for: Dataset Complexity Shapes Finite-Distance Loss Geometry in Neural Networks
Source: arXiv:2608.22361 source file (2026-08-23)
Supplement: Supplementary file 1 [file supplementary.tex]

\documentclass[aps,pre,preprint,superscriptaddress,longbibliography]{revtex4-2}

\usepackage[T1]{fontenc}
\usepackage[utf8]{inputenc}
\usepackage{lmodern}
\usepackage{amsmath,amssymb,bm,mathtools}
\usepackage{graphicx}
\usepackage{booktabs}
\usepackage{microtype}
\usepackage{xcolor}
\usepackage[colorlinks=true,allcolors=blue!55!black]{hyperref}
\hypersetup{
pdftitle={Supplementary Material}, pdfauthor={Jaeyong Bae and Hawoong Jeong}
}

\begin{document}
\input{sections/12_replica_supplement}
\end{document}
